# Supplementary material for: Contact area of rough spheres: Large scale simulations and simple scaling laws
Source: arXiv:1508.02154 ancillary file (2016-06-02)
Supplement: Supplementary file 1 [file supporting_material.pdf]

# Supplemental Material for
# "Simple scaling laws for contact area of rough spheres"

Lars Pastewka[1,2] and Mark O. Robbins[2]

[1] Institute for Applied Materials, Karlsruhe Institute of Technology,
Engelbert-Arnold-Straße 4, 76131 Karlsruhe, Germany

[2] Department of Physics and Astronomy, Johns Hopkins University,
3400 North Charles Street, Baltimore, MD 21218, USA

## S-1. Self-affine, randomly rough surfaces

We create random surfaces of periodic linear length $L$ with Hurst exponent $H$ and self-affine scaling between wavelength $\lambda_s$ and $\lambda_L$. Self-affine scaling implies that height fluctuations $\delta h$ between two points separated by a distance $l$ scale as $\delta h \propto l^H$. The power-spectral density of a surface $C(q_x, q_y) \equiv |\tilde{h}(q_x, q_y)|^2$, where $\tilde{h}(q_x, q_y)$ is the Fourier transform of the heights $h(x, y)$. For isotropic surfaces $C(q_x, q_y) = C(q)$, where q is the magnitude of the wavevector $\vec{q}$. For self-affine surfaces, $C(q)$ follows the power-law expression

$$C(q) \propto q^{-2-2H} \qquad \text{(S-1)}$$

between wavevectors $q_L = 2\pi/\lambda_L$ and $q_s = 2\pi/\lambda_s$ and rolls-off to constant power for $q < q_L$. This behavior is illustrated in Figure S-1. To create these surfaces, we use a Fourier-filtering algorithm [1]. Fourier components for each wavevector have a random phase and a normally distributed amplitude that follows Eq. (S-1).

For a given root mean square slope $(h'_{\text{rms}})^2 \equiv \langle|\nabla h|^2\rangle = (2\pi)^{-1}\int dq\, q^3 C(q)$ the full expression for $C(q)$ for $\lambda_L \gg \lambda_s$ becomes

$$C(q) = 4\pi(1-H)\frac{(h'_{\text{rms}})^2}{q_s^4}\left(\frac{q}{q_s}\right)^{-2-2H} \qquad \text{(S-2)}$$

for $q_L < q < q_s$ and rolls off to $C(q) = C(q_L)$ for $q < q_L$. The root mean square curvature of such a surface is

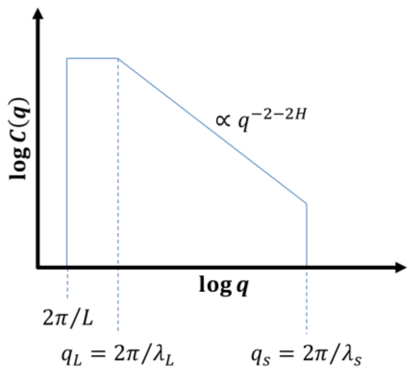


Figure S-1: Sketch of the power spectral density of a self-affine, randomly rough surface with Hurst exponent H and self-affine scaling from wavelength $\lambda_s$ to $\lambda_L$.

$$(h''_{\rm rms})^2 \equiv \langle|\nabla^2 h|^2\rangle = \frac{1}{2\pi}\int dq\, q^5 C(q) = \frac{1-H}{2-H} q_s^2 (h'_{\rm rms})^2 \qquad \text{(S-3)}$$

Using $\rho = 2/h''_{\rm rms}$ gives the expression for the radius of the first contacting asperity quoted in the main text.

## S-2. Effect of interfacial compliance on the dimensionless constant $\kappa$

Figure S-2 illustrates the effect of compliance on the relationship between load and area. The curves represent cross-sections of an elastic substrate intersecting a rigid sphere or cylinder with radius $\rho$. If the interfacial interaction was a hard wall repulsion, the surface displacement would follow the dashed line with radius $\rho$. For a compliant wall at the same contact area, the onset of repulsion is still at the dashed line but the substrate moves downward by a smaller amount (solid line). The difference is largest in the center where the pressure is largest and falls to zero at the edge where the pressure vanishes. The decreased displacement implies a reduction in load at the same area and thus an increase in $\kappa$ to $\kappa_{\rm rep}$.

Our goal is to approximate the effect of compliance as hard wall contact with an effective asperity radius $\rho^{\rm eff}$. The actual substrate profile will be slightly different and depend on the specific form of the interfacial compliance but this simple approximation captures the trends in our numerical results. The displacement from edge to center for the hard wall case is $\delta h = a^2/2\rho$ where $a$ represents the radius of the contact region. To capture the decrease in displacement $c$ at the center of the contact we define $1/\rho^{\rm eff} = 1/\rho - 2c/a^2$. As shown by the solid lines in Figure S-2, this maintains the contact area. The lower load needed to produce this substrate displacement can be calculated from Hertz theory using $\rho^{\rm eff}$. The load scales inversely with radius so the actual load for the compliant surface is smaller by a factor of $\rho/\rho^{\rm eff}$ than predicted by the hard wall expression at the same contact area. This implies

$$\kappa/\kappa_{\rm rep} \equiv \rho/\rho^{\rm eff} = 1 - c/\delta h. \qquad \text{(S-4)}$$

In Ref. [2] we examined the geometry of the contact area in the regime where area is proportional to load. One finds that the diameter of the contact $d_{\rm rep} = 2a = 4\, h'_{\rm rms}/h''_{\rm rms}$ [2] depends only on surface slope and curvature and is independent of load and interaction range. Using Eq. (S-3) we find

$$d_{\rm rep} = 4\lambda_s/2\pi\sqrt{(1-H)/(2-H)}. \qquad \text{(S-5)}$$

For hard wall interactions, the contact mechanics are captured by a locally cylindrical geometry with

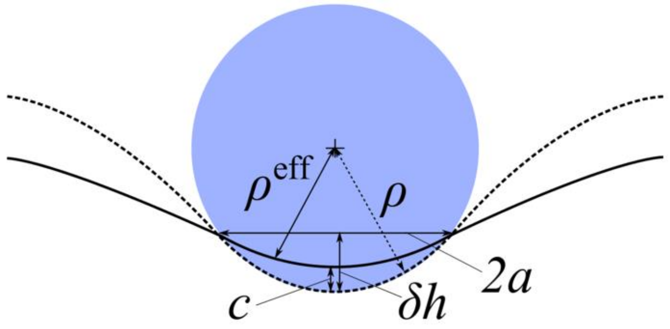


Figure S-2: Sphere or cylinder contacting an elastic substrate. The dashed lines illustrate the substrate deformation for hard-wall repulsive interaction where the cyclinder cannot penetrate the substrate. The solid lines sketches the deformation with a compliant potential for a sphere or cylinder making contact with the same diameter $2a$ as the hard-wall case.

$\delta h = h'_{\mathrm{rms}} d_{\mathrm{rep}}/4$ since the slope sets the typical height change in the contact. For compliant surfaces we calculate $c$ assuming it is proportional to the mean pressure in the contact: $c = N/kA = h'_{\mathrm{rms}} E^*/k\kappa_{\mathrm{rep}}$, where $k$ is the stiffness of the potential per unit area. Substituting into Eq. (S-4) and rearranging the terms gives:

$$\kappa_{\mathrm{rep}} = \kappa + 4E^*/kd_{\mathrm{rep}} \tag{S-6}$$

The local pressure $p(z)$ produced by interfacial potential used in the numerical calculations is

$$p(z) = \frac{k}{a_0^2} \begin{cases} \frac{a_0}{6}\left[\left(\frac{a_0}{z}\right)^{10} - \left(\frac{a_0}{z}\right)^{4}\right] & \text{if } z \le a_0 \\ -(z-a_0) + \frac{2}{\Delta r}(z-a_0)^2 - \frac{1}{\Delta r^2}(z-a_0)^3 & \text{if } a_0 < z < a_0 + \Delta r \\ 0 & \text{if } z \ge a_0 + \Delta r \end{cases} \tag{S-7}$$

where $z = a_0 - c$ is the distance between the two interacting surfaces and $a_0$ is the grid spacing of the deformable half-space. This potential has $k = \partial p/\partial z = E^*/2a_0$ at $z = a_0$ ($c = 0$). The interaction range $\Delta r$ controls the work of adhesion $w$ at constant $k$.We get $\Delta r = 0$, $\Delta r = 0.165a_0$ and $\Delta r = 0.346$ for $w = 0$, $w/E^* = 0.0005a_0$ and $w/E^* = 0.005a_0$ used in our simulations.

The surface roughness has $\lambda_s = 4a_0$, $H = 0.8$ and $d_{\mathrm{rep}} \approx 6.2a_0$, which gives a value of $\kappa_{\mathrm{rep}} = 3.3$ from Eq. (S-6). A fully self-consistent solution of Eq. (S-4) that considers the increase in stiffness $k$ with $c$ given by Eq. (S-7) gives the value of $\kappa_{\mathrm{rep}} = 2.9$ quoted in the main text. Calculated values for $\kappa_{\mathrm{rep}}$ from past studies [3,4] give results that are qualitatively consistent with Eq. (S-6). In particular the value of $\kappa_{\mathrm{rep}}$ goes up as the interface becomes more compliant or the short wavelength cutoff in the roughness decreases.

## S-3. References


[1] S. B. Ramisetti, C. Campañá, G. Anciaux, J.-F. Molinari, M. H. Müser, and M. O. Robbins, J. Phys. Condens. Matter **23**, 215004 (2011).

[2] L. Pastewka and M. O. Robbins, Proc. Natl. Acad. Sci. U. S. A. **111**, 3298 (2014).

[3] M. H. Müser, Phys. Rev. Lett. **100**, 55504 (2008).

[4] S. Akarapu, T. Sharp, and M. O. Robbins, Phys. Rev. Lett. **106**, 204301 (2011).
